# Supplementary material for: Taming Pretrained Transformers for Extreme Multi-label Text Classification
Source: arXiv:1905.02331 source file (2020-06-23)
Supplement: Supplementary file 1 [file appendix.tex]

\onecolumn
\section{Datasets and Preprocessing}
\label{app:data}
\begin{table}[h]
    \centering
    \begin{tabular}{c|ccccc}
    \toprule
    Dataset         & $N_{trn}$ & $N_{val}$ & $N_{tst}$ & \#features    & \#labels  \\
    \midrule
    %Reuters21758    & 6,993     & 777       & 3,019     & 23,098        & 90        \\
    \wikis          & 11,265    & 1,251     & 5,732     & 99,920        & 28,139    \\
    \amzcat         & 1,067,616 & 118,623   & 306,782   & 161,926       & 13,234    \\
    %Amazon-1M       & 1,730,292 & 183,835   & 204,139   & 237,847       & 1,056,251 \\
    \bottomrule
    \end{tabular}
    
    \caption{Data Statistics. $N_{trn},N_{val},N_{tst}$ refer to number of
    instances in training, validation, and test set, respectively. The dataset
    is denote as its name, followed by a dash sign, followed by the \#labels.}
    \label{tb:data}
\end{table}
We consider two multi-label text classification datasets downloaded from the publicly
available Extreme Classification Repository ~\cite{extreme_repo} for which we had
access to the full text, namely \wikis and \amzcat. Summary statistics of the
datasets are given in Table \ref{tb:data}. We follow the training and test split
of~\cite{extreme_repo} and set aside $10\%$ of the training instances as the
validation set for hyperparameter tunning. However, since we adhere the text
preprocessing procedure of~\cite{nam2017maximizing}, the data statistics, particularly
the \#labels, would be slightly different from~\cite{extreme_repo}. Specifically,
for raw text input to Seq2Seq-based methods,we replaced numbers with a special
token and then build a word vocabulary using the most frequent 50K words.
Out-of-vocabulary (OOV) words were also replaced with a special token and we
truncated the documents after 300 words.

\wikis This dataset is originally from~\cite{zubiaga2009getting}, made up by
$20,764$ unique English Wikipedia articles with at least $10$ annotations from the
social bookmarking website Delicious. \wikis is widely used in the XMC
literature such as \sleec~\cite{bhatia2015sparse}, \pfastrexml~\cite{jain2016extreme}
and \discmec~\cite{babbar2017dismec}.

\amzcat This dataset is originally from~\cite{mcauley2013hidden},  made up by
the co-purchase review data, along with the ASIN title, descriptions, and categories.
\amzcat is used in the XMC literature such as  \pfastrexml~\cite{jain2016extreme}
and \discmec~\cite{babbar2017dismec}.

\section{Model Architecture}
\begin{figure}[!h]
    \centering
    \includegraphics[width=0.85\textwidth]{figures/secseq_training.png}
    \caption{The proposed \secseq framework.
    Each positive label $\yb_{p_t}$ is represented as a $K$-way $D$-dimensional semantic code
    $\cbb_{p_t} = \{ c_{p_t}^1, \ldots, c_{p_t}^D \}$ via some label compression functions $\phi$.
    We concatenate all positive labels' codes into a longer sequence for training.
    The softmax layer now becomes $O(K)$, which significantly reduces
    model size, speedup training and inference time.}
    \label{fig:seq2seq_compress}
\end{figure}

\begin{figure}[!h]
    \centering
    \includegraphics[width=0.85\textwidth]{figures/secseq_prediction.png}
    \caption{an instance of $\phi(\cdot)$ function using random projection trees.
    Given a label embedding $\vb_l$, several semantic-aware embedding are available such as
    instance indicator vector, word2vec embedding, Fasttext embedding, and more.
    Furthermore, we may consider an ensemble of $M$ random projection trees,
    that leads to a set of $M$ different semantic codes, and train the \secseq
    in parallel without any further cost.}
    \label{fig:label_compress_tree}
\end{figure}

%\section{Additional Results}
